# Supplementary material for: Towards automated sampling of polymorph nucleation and free energies with SGOOP and metadynamics
Source: arXiv:2108.10459 source file (2021-08-24)
Supplement: Supplementary file 1 [file supplement.pdf]

# Supplementary Information: Towards automated sampling of polymorph nucleation and free energies with SGOOP and metadynamics

**Zou, Tsai, and Tiwary**

## I. SGOOP INPUT AND PARAMETERS

SGOOP requires a stationary probability estimate of the system along with dynamical constraint for Maximum Caliber principle. In general, the stationary probability is obtained from long unbiased or biased simulations, in which state-to-state transitions are sampled at least once. In this work, the input trajectory consists of 9 individual metadynamics simulations biasing $S_{\theta_1}$ and $S_{\theta_2}$ for 100 $ns$, concatenated with each other. The stationary probability was then obtained with appropriate reweighting protocol [1]. On the other hand, the dynamical information of the system is obtained from a 500 $ns$ unbiased simulation initiated from liquid state. The probability distribution was constructed using between 20 to 40 bins and the probabilities smaller than a cutoff of $e^{-50}$, i.e., barriers higher than 50 $k_BT$ in free energy, are trimmed to avoid numerical issues. Thus the transition matrices constructed have the same size as the stationary probability distribution.

## II. 1-D REACTION COORDINATE $\chi_4$

As mentioned in main text, we also calculated a 1-d SGOOP RC $\chi_4$. The basinhopping algorithm [3] is applied to search for the maximum of spectral gap space. This optimized RC consisting of four OPs was found as $\chi_4 = 0.5S_{\theta_1} + 0.938S_{\theta_2} - 0.13\theta_1 + 1.00\theta_2$. Fig. 2 shows time series from WTmetaD simualtion along $\chi_4$. Frequent state-to-state transitions are observed at the first 200 $ns$. However the system is trapped in solid state for 200 $ns$ and escapes the well at 480 $ns$. Fig. 2 (b) is the reweighted free energy surface along RC $\chi_4$, where the two basins correspond to liquid and solid states of urea as labeled by the benchmark lines. Fig. 2(c) shows an unreweighted exploration plot in averaged intermolecular angles $\bar{\theta}_1, \bar{\theta}_2$ space demonstrating that four regions are highly explored and they correspond to all four solid states, including initial liquid state (both phases A and IV are located at lower left region (refer landmark in main text for details)). In particular, the upper right region associated with a value of (0.39, 0.93) of $(\bar{\theta}_1, \bar{\theta}_2)$, is urea in phase I. Fig. 2(d) is the reweighted free energy surface and only two wells are observed which are identified as form I and liquid. In summary, biasing $\chi_4$ which excludes $H$ and $N$ does a slightly worse job of sampling than the $\chi_6$ reported in main text.

## III. 1-D REACTION COORDINATE $\chi'_6$

Here we present another 1-d reaction coordinate, $\chi'_6$ optimized using SGOOP with basinhopping algorithm. Similarly, this 1-d reaction coordinate consists of six order parameters, $S_{\theta_1}$, $S_{\theta_2}$, $\bar{\theta}_1$, $\bar{\theta}_2$, $N$, $H$, and is given by $\chi'_6 = -0.787S_{\theta_1} - 0.461S_{\theta_2} - 0.813\bar{\theta}_1 + 1.0\bar{\theta}_2 - 0.383N + 0.076H$. This reaction coordinate has a spectral gap value of 0.2307 under 3-well assumption as shown in Fig. 3 (a), which is slightly lower than the 0.2332 value for $\chi_6$ reported in main text and in next section. Actual coefficients for different order parameters are shown as a bar plot in Fig. 3 (b) and to judge the importance of each component, in Fig. 3 (c) coefficients are rescaled by reweighted standard deviations of input trajectories. Again, entropy order parameters are shown to be the most important features in driving the nucleation process of urea from the melt among other order parameters in the library. Time series of 1-d WTmetaD simulation biasing $\chi'_6$ is shown in Fig. 3 (d) in which transitions from the melt to form I and form IV are observed. From reweighted free energy surface averaged over 3 individual runs shown in Fig. 3 (e), one distinctive barrier between liquid and solid state is sampled and there is no discernible barrier between forms I and IV. Fig. 3 (f) is free energy difference computed with associated landmarks over time. One can also conclude that biasing this slightly sub-optimal SGOOP RC shows correct ranking of polymorph under experimental observations, whereas form I has low free energy than form IV. However, the large discrepancy (in terms of error bars) between the three individual trajectories leads to large uncertainty in Fig. 3 (f), which suggests $\chi'_6$ is a slightly poorer approximation to the reaction coordinate than $\chi_6$ reported main text. Moreover, a large amount of defective structures are sampled while biasing along this reaction coordinate.

## IV. SPECTRAL GAP ANALYSES OF $\chi_6$

The free energy surface along $\chi_6$ through the input trajectories is shown in Fig. 4 (a). Spectral profile of $\chi_6$ is shown in Fig. 4 (b) and the spectral gap equals 0.2332. In Fig. 4 (a), three distinctive wells are identified. By appropriately assigning state labels from landmarks of polymorphs described in main text, the leftmost basin corresponds to form A, the middle one consists of form I and IV, and liquid state locates at the rightmost well. In addition, form B seems to located around transition state between the liquid state and collectively forms I and IV. As shown in Fig. 3 (a), values of spectral gap for $\chi_6$ and $\chi'_6$ are close to each other. But their performances are different. While both gave

correct polymorph ranking, simulations biasing $\chi_6$ with higher spectral gap converged faster than those biasing $\chi_6'$. The $0^{th}$ and $1^{st}$ eigenvectors of the transition matrix are shown in Fig. 4 (c) and (d), respectively, for further analyses. The $0^{th}$ eigenvector has no node and the $1^{st}$ eigenvector has one node located at the transition state of the deepest well, which further suggests $\chi_6$ is a good approximation to the reaction coordinate.

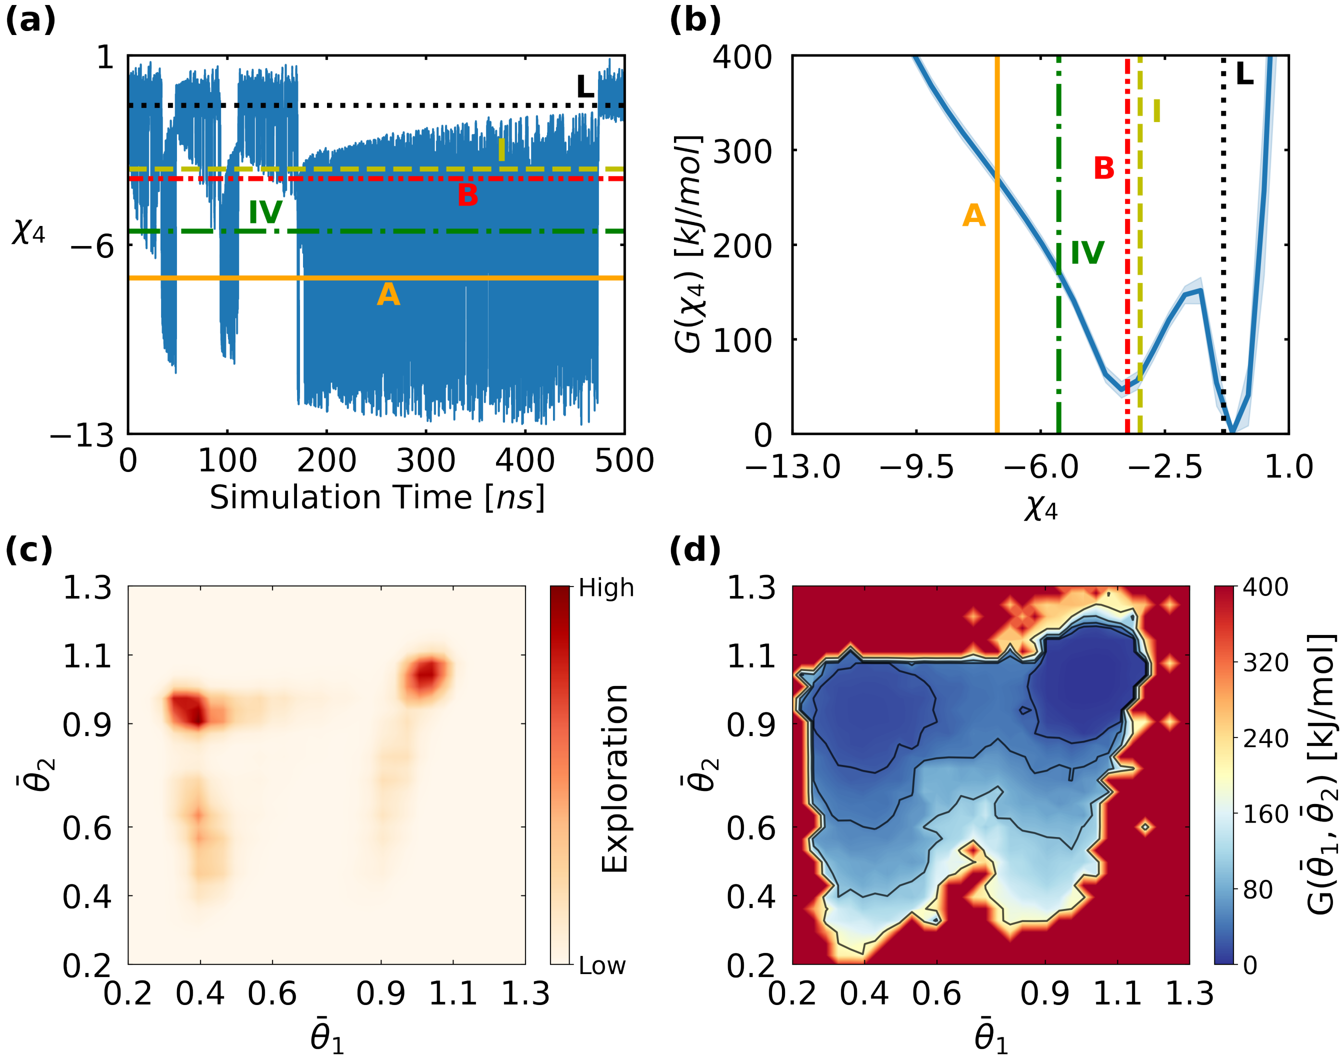


**Supplementary Figure 1:** WTMetaD simulation and thermodynamics analyses: (a) Time series of 1-d WTmetaD biasing $\chi_4$; (b)reweighted free energy surface along $\chi_4$ averaged over 3 individual WTmetaD simulations; (c) unreweighted exploration plot; and (d) reweighted free energy surface in $(\bar{\theta}_1, \bar{\theta}_2)$ space. The benchmark lines of all polymorphs (sampled in Ref. 2) are plotted w.r.t corresponding landmarks (see main text for landmark values). The regions between errorbars are filled with corresponding colors in (b). The exploration plot (c) shows configurations which were frequently visited, and they are form I, IV, A, B and liquid. Reweighted free energy surface (d) presents only the basins of form I and liquid.

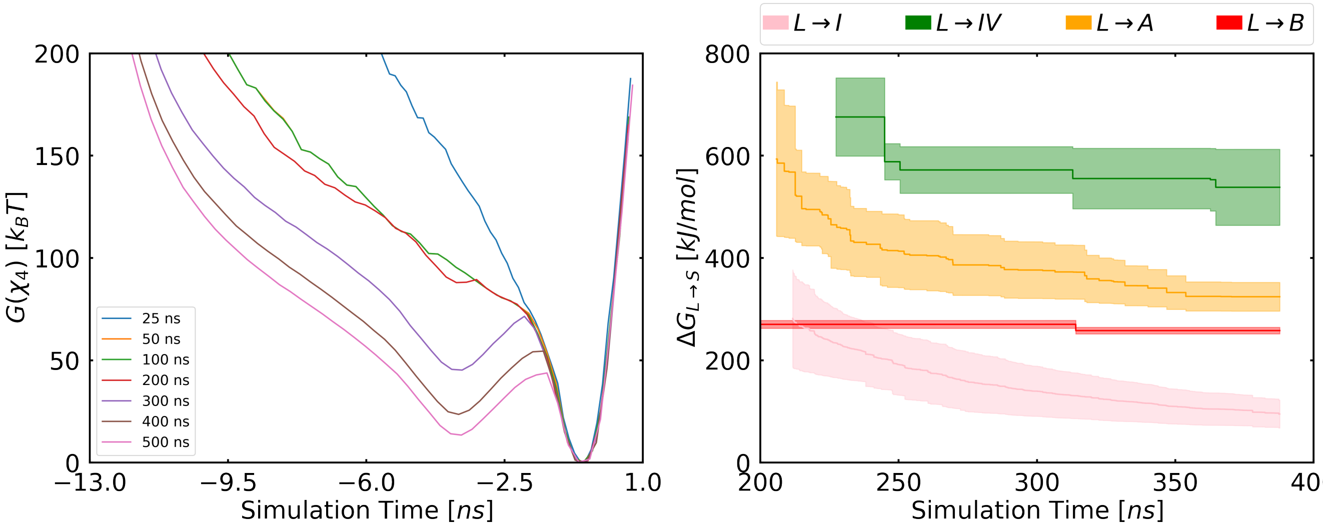


**Supplementary Figure 2:** Convergence check with (a) free energy surface along RC, $\chi_4$, over simulation time and (b) free energy differences of phases averaged over 3 independent trajectories. Error bars are shaded in corresponding colors in (b). Both methods show slow convergence of $\chi_4$.

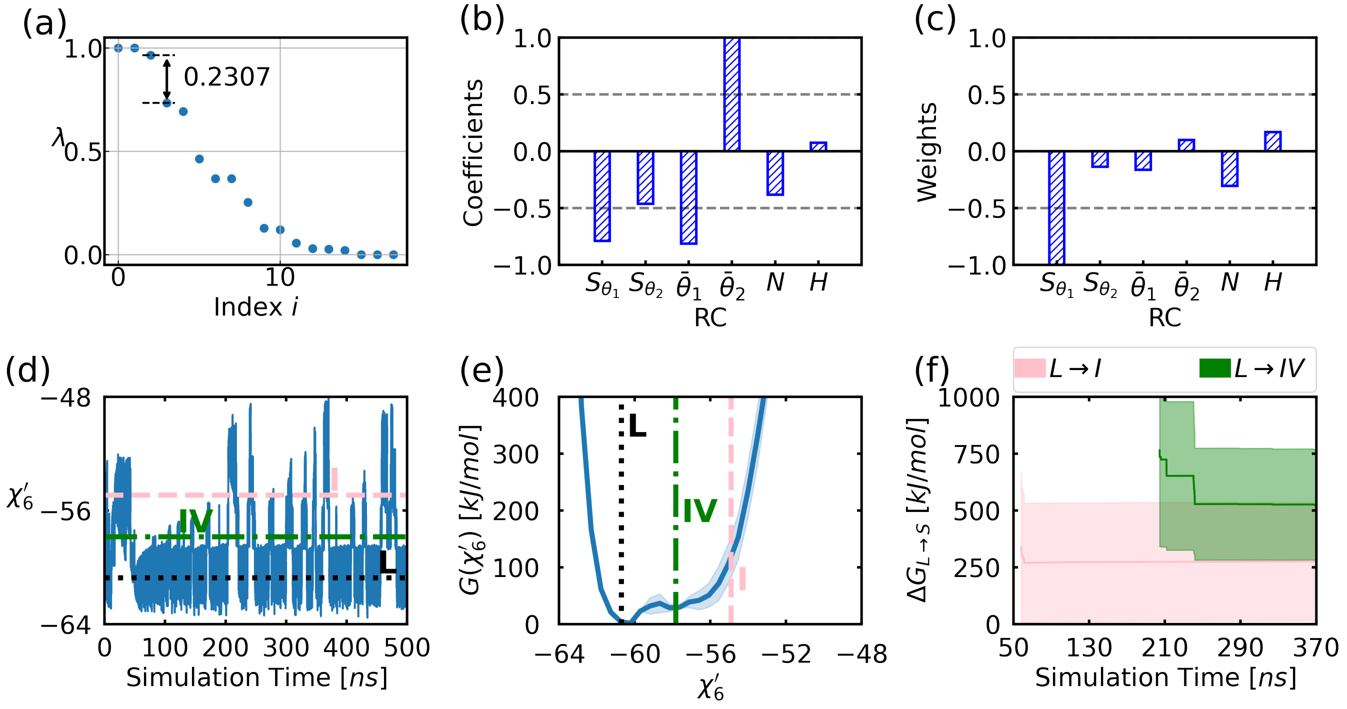


**Supplementary Figure 3:** Details of 1-d SGOOP reaction coordinate $\chi_6'$: a) spectral gap plot of $\chi_6'$ discretized into 20 wells under 3 wells assumption; bar plots for coefficients b) and rescaled weights c) of each order parameters composed in $\chi_6'$; d) time series of $\chi_6'$ with benchmark lines of liquid state (L), form I, and form IV observed with visualization tools; e) reweighted free energy surface along $\chi_6'$; and f) free energy difference of form I and form IV with respect to liquid state over time. Shaded area corresponds to error bars.

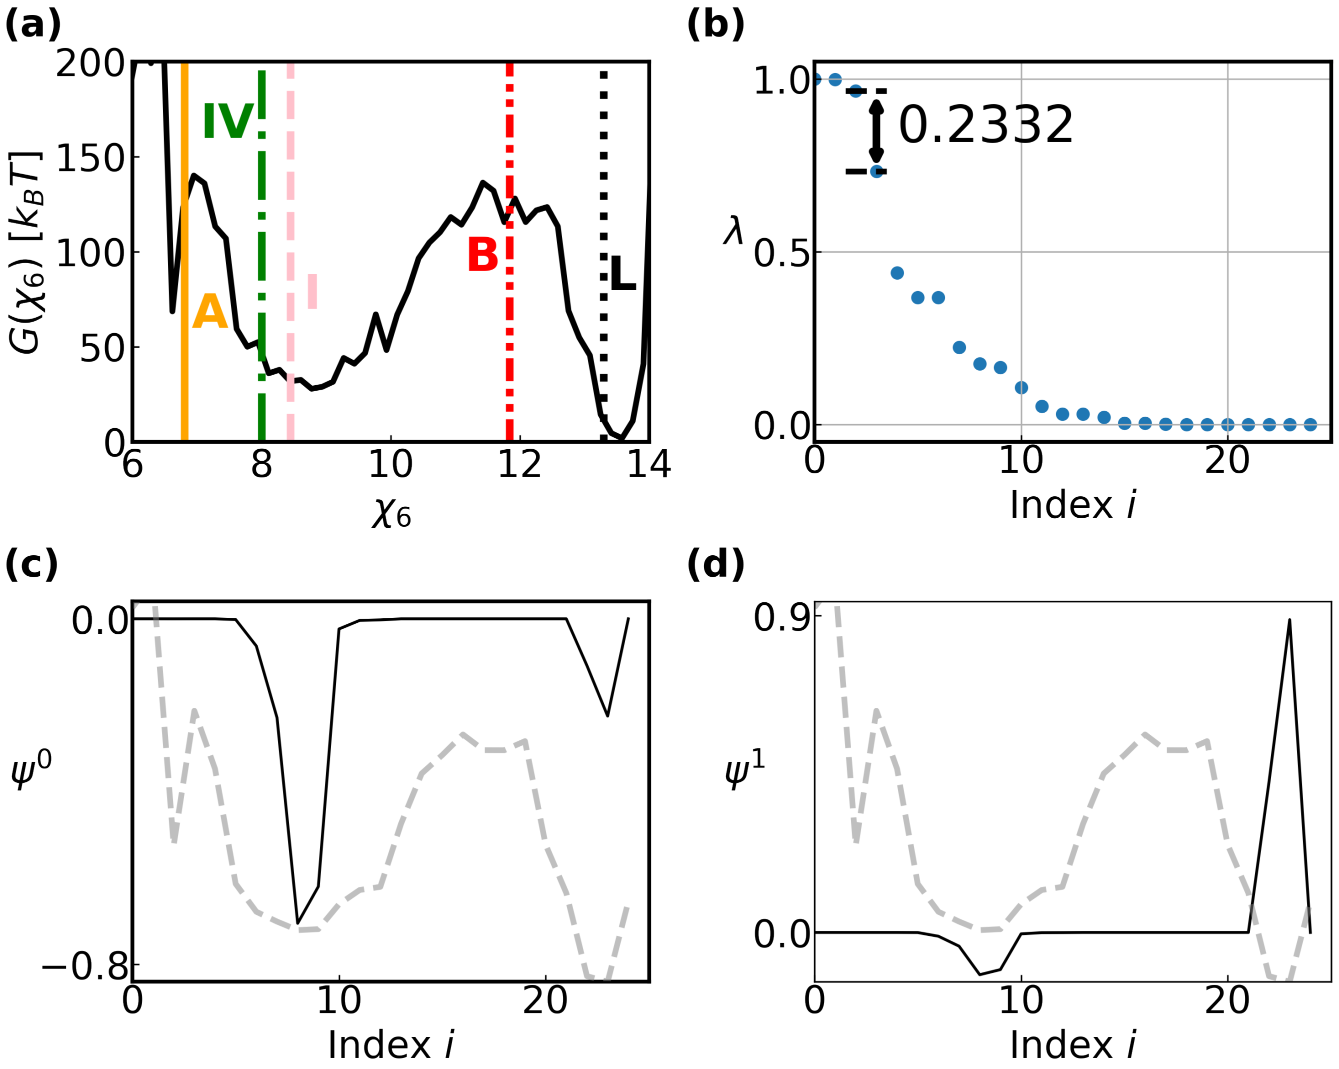


**Supplementary Figure 4:** Spectral gap analyses of $\chi_6$ under 3-well assumption: a) 3 distinctive wells optimized by SGOOP with input data (refer Sec. I for details); b) spectral gap plot constructed from exponential of solved eigenvalues of transition matrix; c) the zeroth and d) the first eigenvectors of obtained transition matrix.

## SUPPLEMENTARY REFERENCES

---

[1] P. Tiwary and M. Parrinello, The Journal of Physical Chemistry B **119**, 736 (2015).
[2] P. M. Piaggi and M. Parrinello, Proceedings of the National Academy of Sciences **115**, 10251 (2018).
[3] D. J. Wales and J. P. K. Doye, The Journal of Physical Chemistry A **101**, 5111 (1997).
